# Supplementary material for: Measurement of Ratios of $\nu_{\mu}$ Charged-Current Cross Sections on C, Fe, and Pb to CH at Neutrino Energies 2-20 GeV
Source: arXiv:1403.2103 source file (2015-03-10)
Supplement: Supplementary file 2 [file biblio-supplement-bibtex.tex]

\bibliographystyle{apsrev4-1}
\bibliography{supplement-NukeCC}
